# Supplementary material for: ASP-based Multi-shot Reasoning via DLV2 with Incremental Grounding
Source: arXiv:2412.17143 source file (2025-04-01)
Supplement: Supplementary file 1 [file appendix.tex]

\appendix
%
% Vecchia appendice con risposte a revisori PPDP ed elenco modifiche della prima versione per rivista.
%

\section{Extended parts of the paper}
The additions and modifications to the paper with respect its version appeared in PPDP2022 proceedings are:
\\

     -- A more detailed introduction to the overgrounding techniques is provided in Section~\ref{sec:overgrounding}.
        
        -- Section~\ref{sec:system} now better clarifies some of the obscure points, as mentioned by reviewers.
        
        -- We introduced pseudocode illustrating how an overgrounded program with tailoring is updated from shot to shot, and modified the implementation description accordingly. 
        
        -- As one of the main issues with overgrounding is the bigger memory usage, we mentioned, whenever appropriate, the presence of a forgetting feature that can help in trimming overgrounded programs if necessary. As this is new research, we refrained from going into technical details.

        -- Section~\ref{sec:usage} has been reorganized and partly rewritten.

        -- We renamed and reorganized Section~\ref{sec:exp+disc} and added informative details as requested by reviewers.

       -- Section~\ref{sec:relwork} is now organized in subsections: it mentions latest state-of-the-art work, and has a new subsection which comments on past publications that presented the formal results supporting our incremental algorithms.

\section{Answers to reviewers of the conference version of this paper}
We thank again the reviewers of the conference version of this paper for their feedback.
As the PPDP paper selection process included a rebuttal step, we report here a revised reply to the questions of reviewers. We did our best to incorporate reviewers feedback, while avoiding to introduce new research, as prescribed by the Rapid Publication policy for TPLP.

\paragraph{\bf Q\&A with Reviewer 1.}

Many thanks for your general appreciation of the paper. 
\\
\\
{\em How the system decides which simplifications to undo?}

Thanks for the question. The paper now better clarifies how the simplification and desimplification mechanism is performed. Basically, at each shot, the system stores all generated ground rules in their complete and non-simplified version along with information (i.e.,  meta-data) regarding body literals that are simplified and ground rules that are simplified (e.g., those containing a certainly false literal in the body). Such rules are possibly desimplified in the next shots, and, taking into account the information on the occurred simplifications, 1) no longer certainly true body literals are restored and 2) rules that have been simplified because of a false literal in their body are restored.
\\
\\
{\em  The section on experimental evaluation, besides
being oddly named, gives three practical example scenarios stemming
from the same group at UniCal.}

We renamed Section~\ref{sec:exp+disc}.
\\
\\
{\em 
The experimental evaluation states what hardware was used for the
timings, but omits to clarify whether the runs were single-threaded or
if they used all the available cores.
When comparing with regular DLV2, it is unclear whether the base
process also has to be restarted (i.e. is the process in a loop or
does this have to be conducted in a shell process of some kind?)}
\\
We added all the missing details to Section~\ref{sec:system}.
The runs were single-threaded: the sub-systems of the new system stay alive and run in a single process, indeed they
share many data structures which allow to avoid piping data from one shell process to another. The regular DLV2 is restarted from shot to shot.
\\
\\
{\em 
The performance characterization of both Incremental-DLV2 and DLV2
takes up most of a page in graphics which don't really convey much
information.  It would be better to indicate, instead of runtimes and
megabytes, a base time and a speedup (e.g. the DLV2 measure would be
the reference and the Incremental-DLV2 would be presented as a factor,
e.g. 10% or 2*) - straight timing graphs are difficult to interpret.
Also, the plateau in the pacman memory use is asking for a better
explanation.}

We revised the layout of graphs. Concerning the speedup factors and memory growth, we reported about in text.
We better detailed how the memory use behaves in pacman.
\\
\\
{\em
W.r.t. the possible future work, the "automated forgetfulness" sounds
interesting but it is not clear how much of the "old" clauses actually
contributes to memory use.  Maybe an investigation of the sources of
memory use would be more beneficial.
}

We agree. We are currently working on that: one of our early contributions about is \cite{DBLP:conf/padl/CalimeriIPPZ24}. We added some information on how our forgetting works, although we couldn't go in more detail as we cannot add new research here.
\\
\paragraph{\bf Q\&A with Reviewer 2.}
Many thanks for your general appreciation of the paper.
\\
\\
{\em In other words, besides the use of $I^2$-$DLV$, what were the challenges in the development of Incremental-DLV2?}

Thanks for the question. Section \ref{sec:system} now clarifies that Incremental-DLV2 integrates $I^2$-$DLV$ as grounding sub-system that  implements overgrounding techniques as a way to enable incrementality in the computation. On the solving side, Incremental-DLV2 relies on the same non-incremental solving algorithms adopted in DLV2. However, differently from DLV2, both the grounding and the solving sub-systems are now kept alive across the shots; while $I^2$-$DLV$ was already designed to this extent, the solving subsystem has been modified to remain alive as well. 
Also we moved from a loose coupling architecture, where the two subsystems were sharply separated, to a tighter coupling, in which some data structures are shared, and thus they do not need to be piped from a system to another at each iteration.
The solver performs the evaluation only on a relevant portion of the overgrounded program that is efficiently passed via these shared internal data-structures updated from shot to shot. 
\\
\\
{\em The description is perhaps a bit too verbose.
An algorithm would be easier to grasp.}

We added pseudocode for the internal algorithm implementing overgrounding with tailoring in Figure~\ref{alg:simplinf} and changed the text description accordingly.

\paragraph{\bf Q\&A with Reviewer 3.}
Many thanks for your general appreciation of the paper.
